# Supplementary material for: Beyond Newton: a new root-finding fixed-point iteration for nonlinear equations
Source: arXiv:1803.10156 source file (2018-07-11)
Supplement: Supplementary file 1 [file si.pdf]

# Supplementary Information

Beyond Newton: a new root-finding fixed-point iteration for nonlinear equations

Ankush Aggarwal, Sanjay Pant

## 1 Inverse of $x$

We consider a function

$$r(x) = \frac{1}{x} - H, \tag{S1}$$

which is discontinuous at $x = 0$. The convergence behavior using three methods are shown (Figs. S1–S3), where discontinuity leads to non-smooth results.

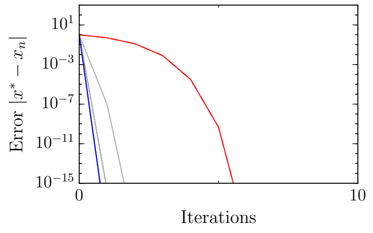


Figure S1: Convergence of Eq. (S1) using standard Newton (red), Extended Newton (gray), and Corrected Newton (blue) methods for $H = 0.5$, $x_0 = 1$, and $c \in (1, 50)$

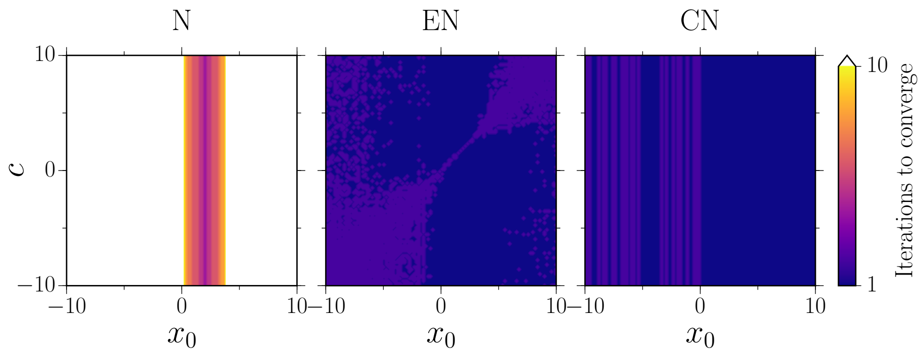


Figure S2: Iterations to converge for Eq. (S1) using (from left) standard Newton, Extended Newton, and Corrected Newton methods for $H = 0.5$ and varying $x_0$ and $c$

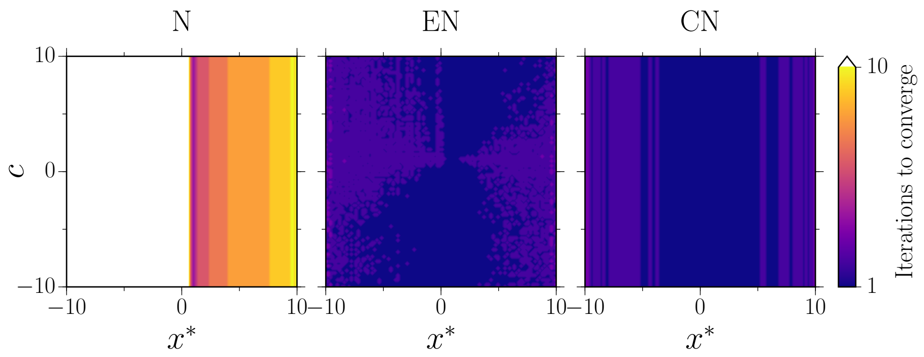


Figure S3: Iterations to converge for Eq. (S1) using (from left) standard Newton, Extended Newton, and Corrected Newton methods for $x_0 = 1$ and varying $x^*$ and $c$

# 2 Nonlinear compression

We consider a function from nonlinear elasticity, which is only defined in $\mathbb{R}^+$:

$$r(x) = \begin{cases} x^2 - \frac{1}{x} + H & \text{if } x > 0 \\ \text{Not defined} & \text{if } x \leq 0 \end{cases} . \tag{S2}$$

If the current guess $x_n$ becomes negative, the iterations are considered to be non-converged. The resulting convergence behavior is shown (Fig. S4–S6)

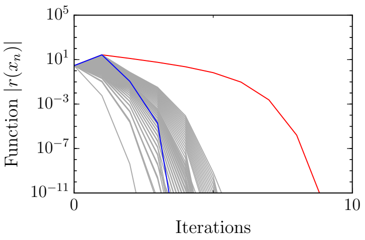


Figure S4: Convergence of Eq. (S2) using standard Newton (red), Extended Newton (gray), and Corrected Newton (blue) methods for $H = 2.9$, $x_0 = 1$, and $c \in (0.01, 1)$

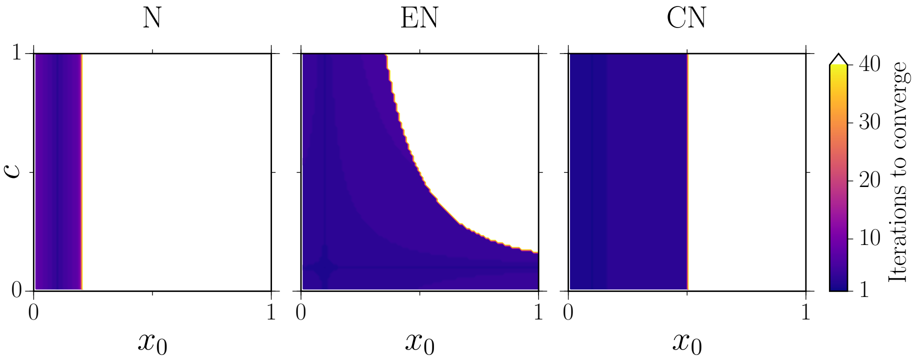


Figure S5: Iterations to converge for Eq. (S2) using (from left) standard Newton, Extended Newton, and Corrected Newton methods for $H = 10$ and varying $x_0$ and $c$

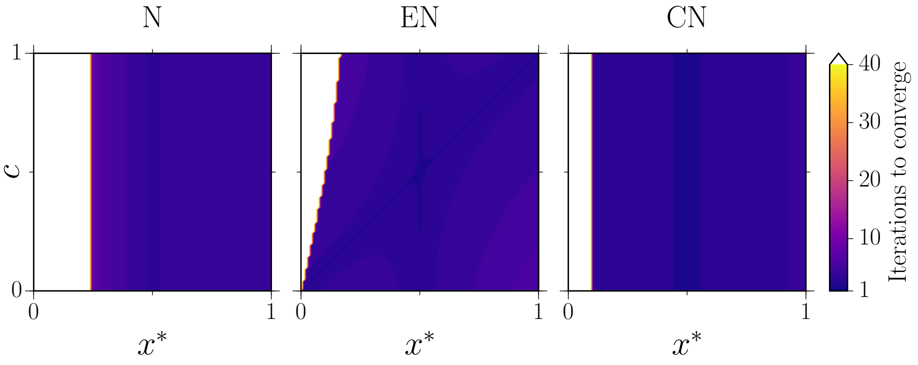


Figure S6: Iterations to converge for Eq. (S2) using (from left) standard Newton, Extended Newton, and Corrected Newton methods for $x_0 = 0.5$ and varying $x^*$ and $c$

## 3 Transcendental equation

We consider the following transcendental equation with restricted domain

$$r(x) = \begin{cases} \tan(x) - x & \text{if } x \in [\pi, 3\pi/2] \\ \text{Not defined} & \text{if } x < \pi \text{ or } x > 3\pi/2 \end{cases} . \tag{S3}$$

If the current guess goes outside the domain ($x_n < \pi$ or $x_n > 3\pi/2$), the iterations are considered to be non-converged. Resulting convergence behavior is shown (Fig. S7).

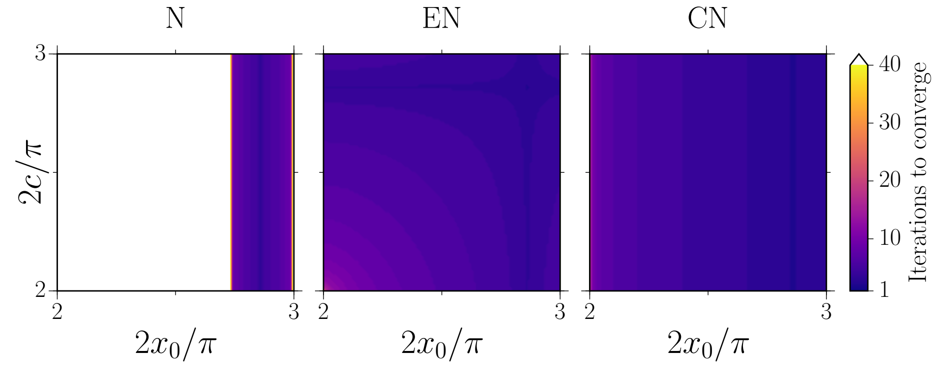


Figure S7: Iterations to converge for Eq. (S3) using (from left) standard Newton, Extended Newton, and Corrected Newton methods for varying $x_0$ and $c$

## 4 Dimension of Newton Fractal

For the Newton fractal for $r(z) = z^3 - 1$ (Fig. 3, main manuscript), we calculate the dimension of the boundary between basins of attraction (i.e. Julia set) using box counting method (Fig. S8).

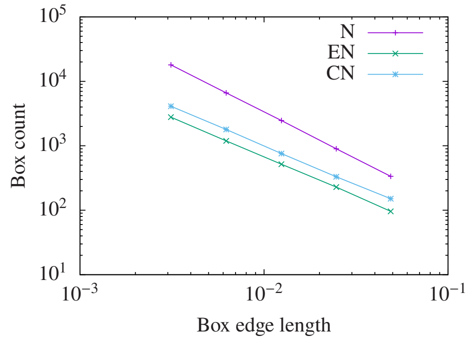


Figure S8: Dimension $d$ of the boundary between basins of attraction for $r(z) = z^3 - 1$ calculated by box counting: $d \approx 1.45$ for standard Newton's method, $d \approx 1.22$ for Extended Newton method with $c = -0.65 - 0.65i$, and $d \approx 1.20$ for Corrected Newton method
